# Supplementary material for: `Why didn't you allocate this task to them?' Negotiation-Aware Explicable Task Allocation and Contrastive Explanation Generation
Source: arXiv:2002.01640 source file (2023-05-25)
Supplement: Supplementary file 1 [file appendices.tex]

\documentclass{article}

\usepackage[utf8]{inputenc}
\usepackage[final]{pdfpages}
\usepackage{xcolor}
% Use the postscript times font!

\usepackage{soul}
\usepackage{url}
\usepackage[hidelinks]{hyperref}
\usepackage[utf8]{inputenc}
\usepackage{caption}
\usepackage{graphicx}
\usepackage{amsmath}
\usepackage{amsthm}
\usepackage{booktabs}
\usepackage{algorithm}
\usepackage{algorithmic}
\usepackage[switch]{lineno}
\usepackage{soul}
\usepackage{tikz}
\usepackage{pgfplots} 
\usetikzlibrary{pgfplots.dateplot}
\usepackage{pgfplotstable}
\usepackage{filecontents}
\usepackage{balance}
\usepackage{booktabs}
\usepackage{adjustbox}

\usepackage{amssymb}

% ...
\begin{document}
\begin{center}
\section*{Appendix A -- Average scores of Different Explanations}
The average scores for understanding and convincing of the three explanations in the relative case of the human studies are given in the following table.
\begin{table}[h]
\centering
\caption{Human study scores for our negotiation-tree based explanations compared to the two baselines.}
\label{tab:relative}
\begin{tabular}{llcc}
\toprule
Domain & Explanation & Understandable & Convincing \\
& & $(1-5)$ & $(1-5)$\\
\cmidrule{2-4}
Cooking & Vacuous & 4.5 & 2.33 \\
& Verbose & 4.3 & 4 \\
& Neg-tree & 4.5 & 4 \\
\cmidrule{2-4}
Class & Vacuous & 4.4 & 2.8 \\
Project & Verbose & 4.2 & 3.4 \\
& Neg-tree & 3.8 & 4.4 \\
\bottomrule
\end{tabular}
%\vspace{-0.55cm}
\end{table}
\section*{Appendix B -- Costs for Project Management Scenario}
Agent's true costs for completing each of the five tasks is provided in the following Table.\\
\begin{table}[h]
\centering
\caption{Agent's true costs for completing a task.}
\label{tab:agent_cost}
\begin{tabular}{lccccc}
\toprule
        & $t_1$ & $t_2$ & $t_3$ & $t_4$ & $t_5$ \\
\midrule
$1$ & $0.3$    & $0.5$    & $0.4$    & $0.077$  & $0.8$    \\
$2$ & $0.4$    & $0.7$    & $0.077$  & $0.49$   & $0.13$  \\
\bottomrule
\end{tabular}
%\vspace{-0.55cm}
\end{table}

Also the $32$ (true) costs for team performance shown below.

{\tt
\noindent 1.812 1.7597 1.82705 1.77475 2.00005 1.94775 2.0151 1.9628 2.16 2.1077 2.17505 2.12275 2.34805 2.29575 2.3631 2.3108 2.17005 2.11775 2.1851 2.1328 2.3581 2.3058 2.37315 2.32085 2.51805 2.46575 2.5331 2.4808 2.7061 2.6538 2.72115 2.6685
}
\section*{Appendix C -- Human Study details}
We provide the details of the three task-allocation experiments considered in the human subject studies.
\newpage
\subsection*{Cooking Domain}
\newpage
% includes all pages in the pdf
\includepdf[pages=-]{HS-files/cooking.pdf}

% includes pages 1, 2 and 4 of the pdf

\subsection*{Team Project Domain}
\newpage
\includepdf[pages=-]{HS-files/project.pdf}

\subsection*{Paper Domain}
\newpage
\includepdf[pages=-]{HS-files/paper.pdf}

\end{center}
% ...
\end{document}
